# Supplementary material for: Do Neural Networks Generalize from Self-Averaging Sub-classifiers in the Same Way As Adaptive Boosting?
Source: arXiv:2302.06923 source file (2023-02-14)
Supplement: Supplementary file 1 [file 0suppl_text.tex]

\subsection*{Supplemental Text}

Some supplemental text that doesn't fit in the main text or provides extra detail can go here. We will use this space to outline some general tips.

\subsubsection*{Article tips, tricks, and nitpicks}
\generalTips
