# Supplementary material for: Do Neural Networks Generalize from Self-Averaging Sub-classifiers in the Same Way As Adaptive Boosting?
Source: arXiv:2302.06923 source file (2023-02-14)
Supplement: Supplementary file 2 [file 1suppl_figs.tex]

\subsection*{Supplemental Figures}
\setcounter{figure}{0} % set figs to start at 1
 % start figures with "S"

% See 4maintextFigs.txt for functions and usage to help streamline making figures

%%%% tony %%%%

\generateFig{tony}{tony}{.3} 
    {This is a picture of Tony Capra.} % bold caption
    {Nobody puts Tony in a supplement\dots} % unbold caption
\tony

%%%% cutegoat %%%%
% Example of sideways figure

\generateFig[90]{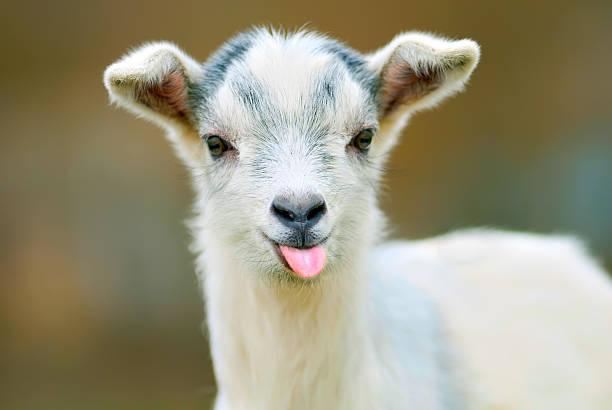}{cutegoat}{.6} % Make angle 90deg
    {This cute sideways goat wishes you good luck with your manuscript.} % bold caption
    {This is how you rotate a figure but not the caption. To rotate the caption with the figure, use the function(s) \texttt{generateSidewaysFig} or \texttt{generateSidewaysFigSubpanels}.} % unbold caption
\cutegoat

\clearpage
