# Supplementary material for: Do Neural Networks Generalize from Self-Averaging Sub-classifiers in the Same Way As Adaptive Boosting?
Source: arXiv:2302.06923 source file (2023-02-14)
Supplement: Supplementary file 3 [file 2suppl_tabs.tex]

\subsection*{Supplemental Tables}
\setcounter{table}{0} % set tables to start at 1
 % start tables with "S"

%%%% sampleTable %%%%

\generateTab{sampleTable}{supplement/suppl_tabs/sampleTable}{.55}
    {Example table.} % Main caption
    {I use \texttt{Excel2LaTeX.xla} to create easy tables. There are also other online websites. Look for one that is booktabs enabled. Here's good advice about making simple readable tables: \url{https://users.umiacs.umd.edu/~jbg/images/tables.gif}} % Small caption
\sampleTable

% Example of how to make a sideways table
% \generateSidewaysTab{sampleTableSideways}{supplement/suppl_tabs/sampleTable}{.3}
%     {Sideways Table.} % Main caption
%     {Wow! This might be really useful for tables with lots of columns and fewer rows.} % Small caption
% \sampleTableSideways

\clearpage
